# Supplementary material for: Temperature and Pressure Dependent Vibrational Properties of Pristine and Doped Vacancy-Ordered Double Perovskite
Source: arXiv:2512.21810 source file (2025-12-31)
Supplement: Supplementary file 1 [file appendixA.tex]

\chapter{Experimental Setup\label{cha:appendix}}

\begin{figure}[h]
\begin{center}
 \includegraphics[scale = 0.09]{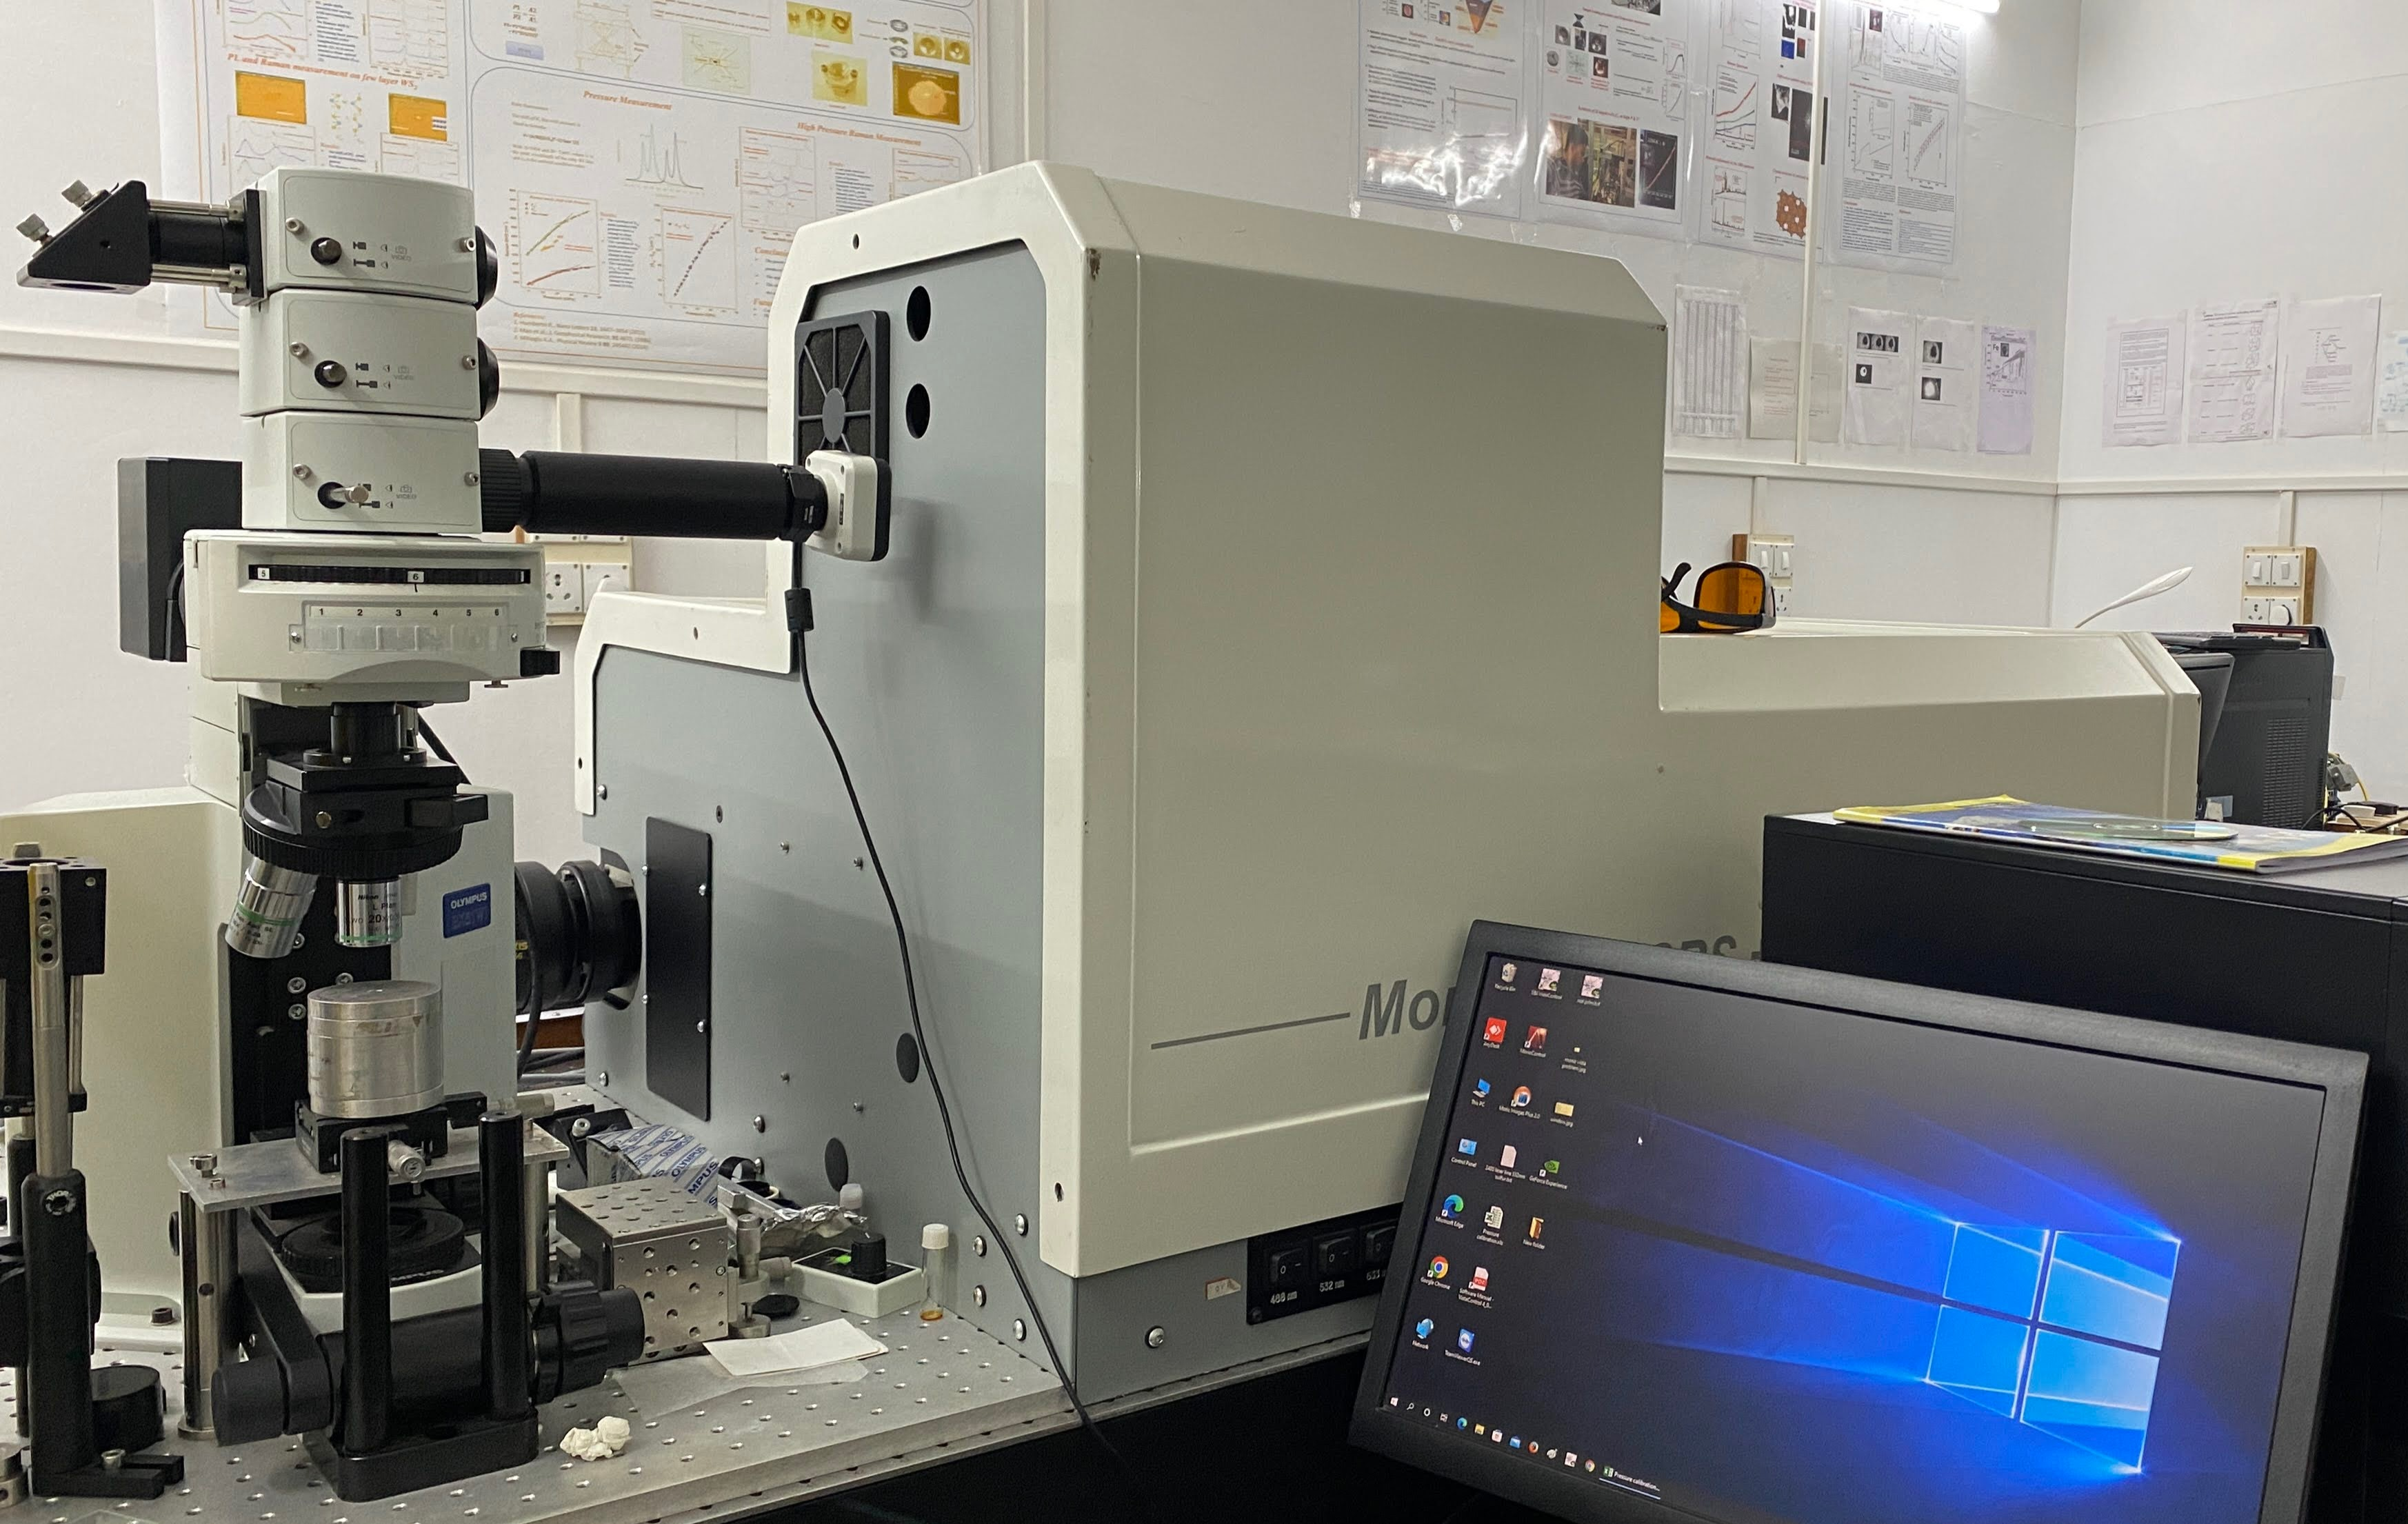}   
 \caption{Micro Raman spectrometer setup}
 \label{fig:my_label}
\end{center}
\end{figure}

\begin{figure}[h]
\centering
\begin{subfigure}{0.4\textwidth}
    \includegraphics[width=\textwidth]{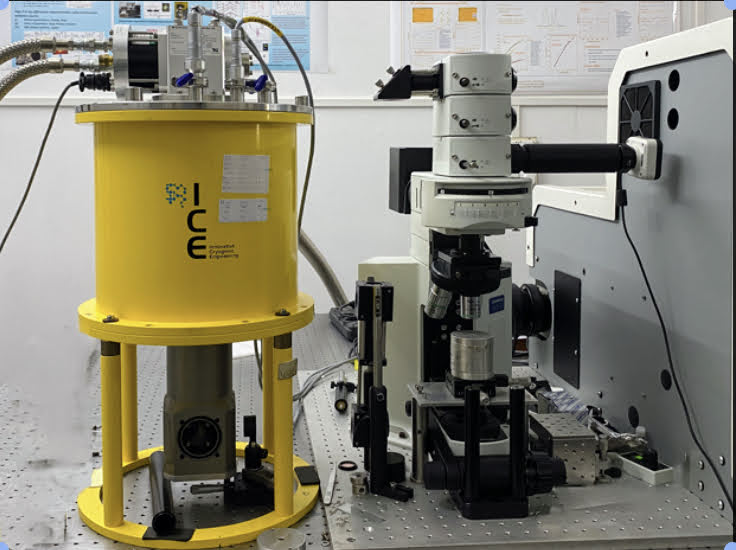}
    \caption{Low temperature Raman setup}
    \label{fig:first}
\end{subfigure}
\hfill
\begin{subfigure}{0.2\textwidth}
    \includegraphics[width=\textwidth]{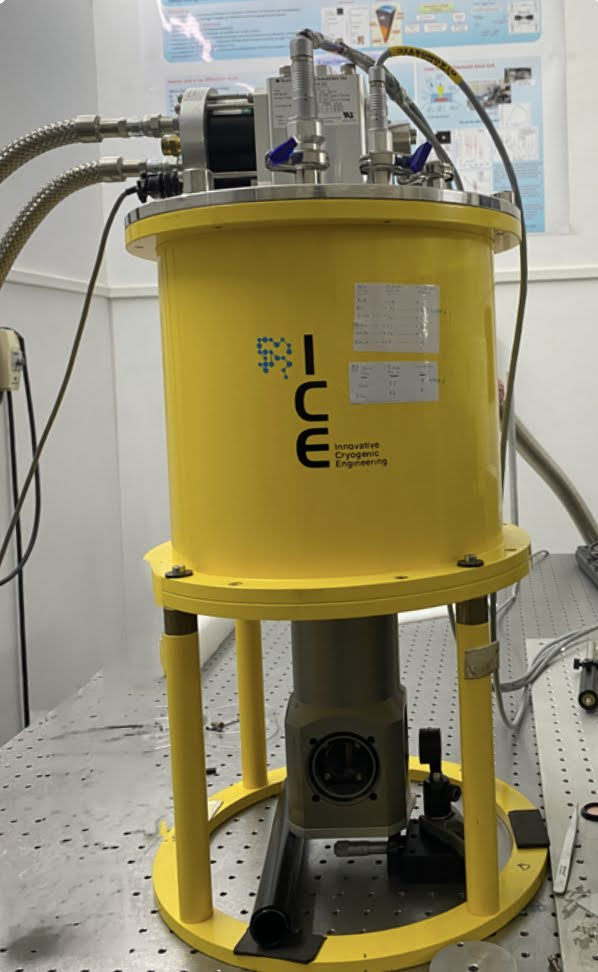}
    \caption{Helium cooled Cryostat}
    \label{fig:second}
\end{subfigure}
\hfill
        
\caption{Low temperature Raman setup with Helium cooled Cryostat}
\label{fig:figures}
\end{figure}

\begin{figure}[h]
\begin{subfigure}{0.44\textwidth}
    \includegraphics[width=\textwidth]{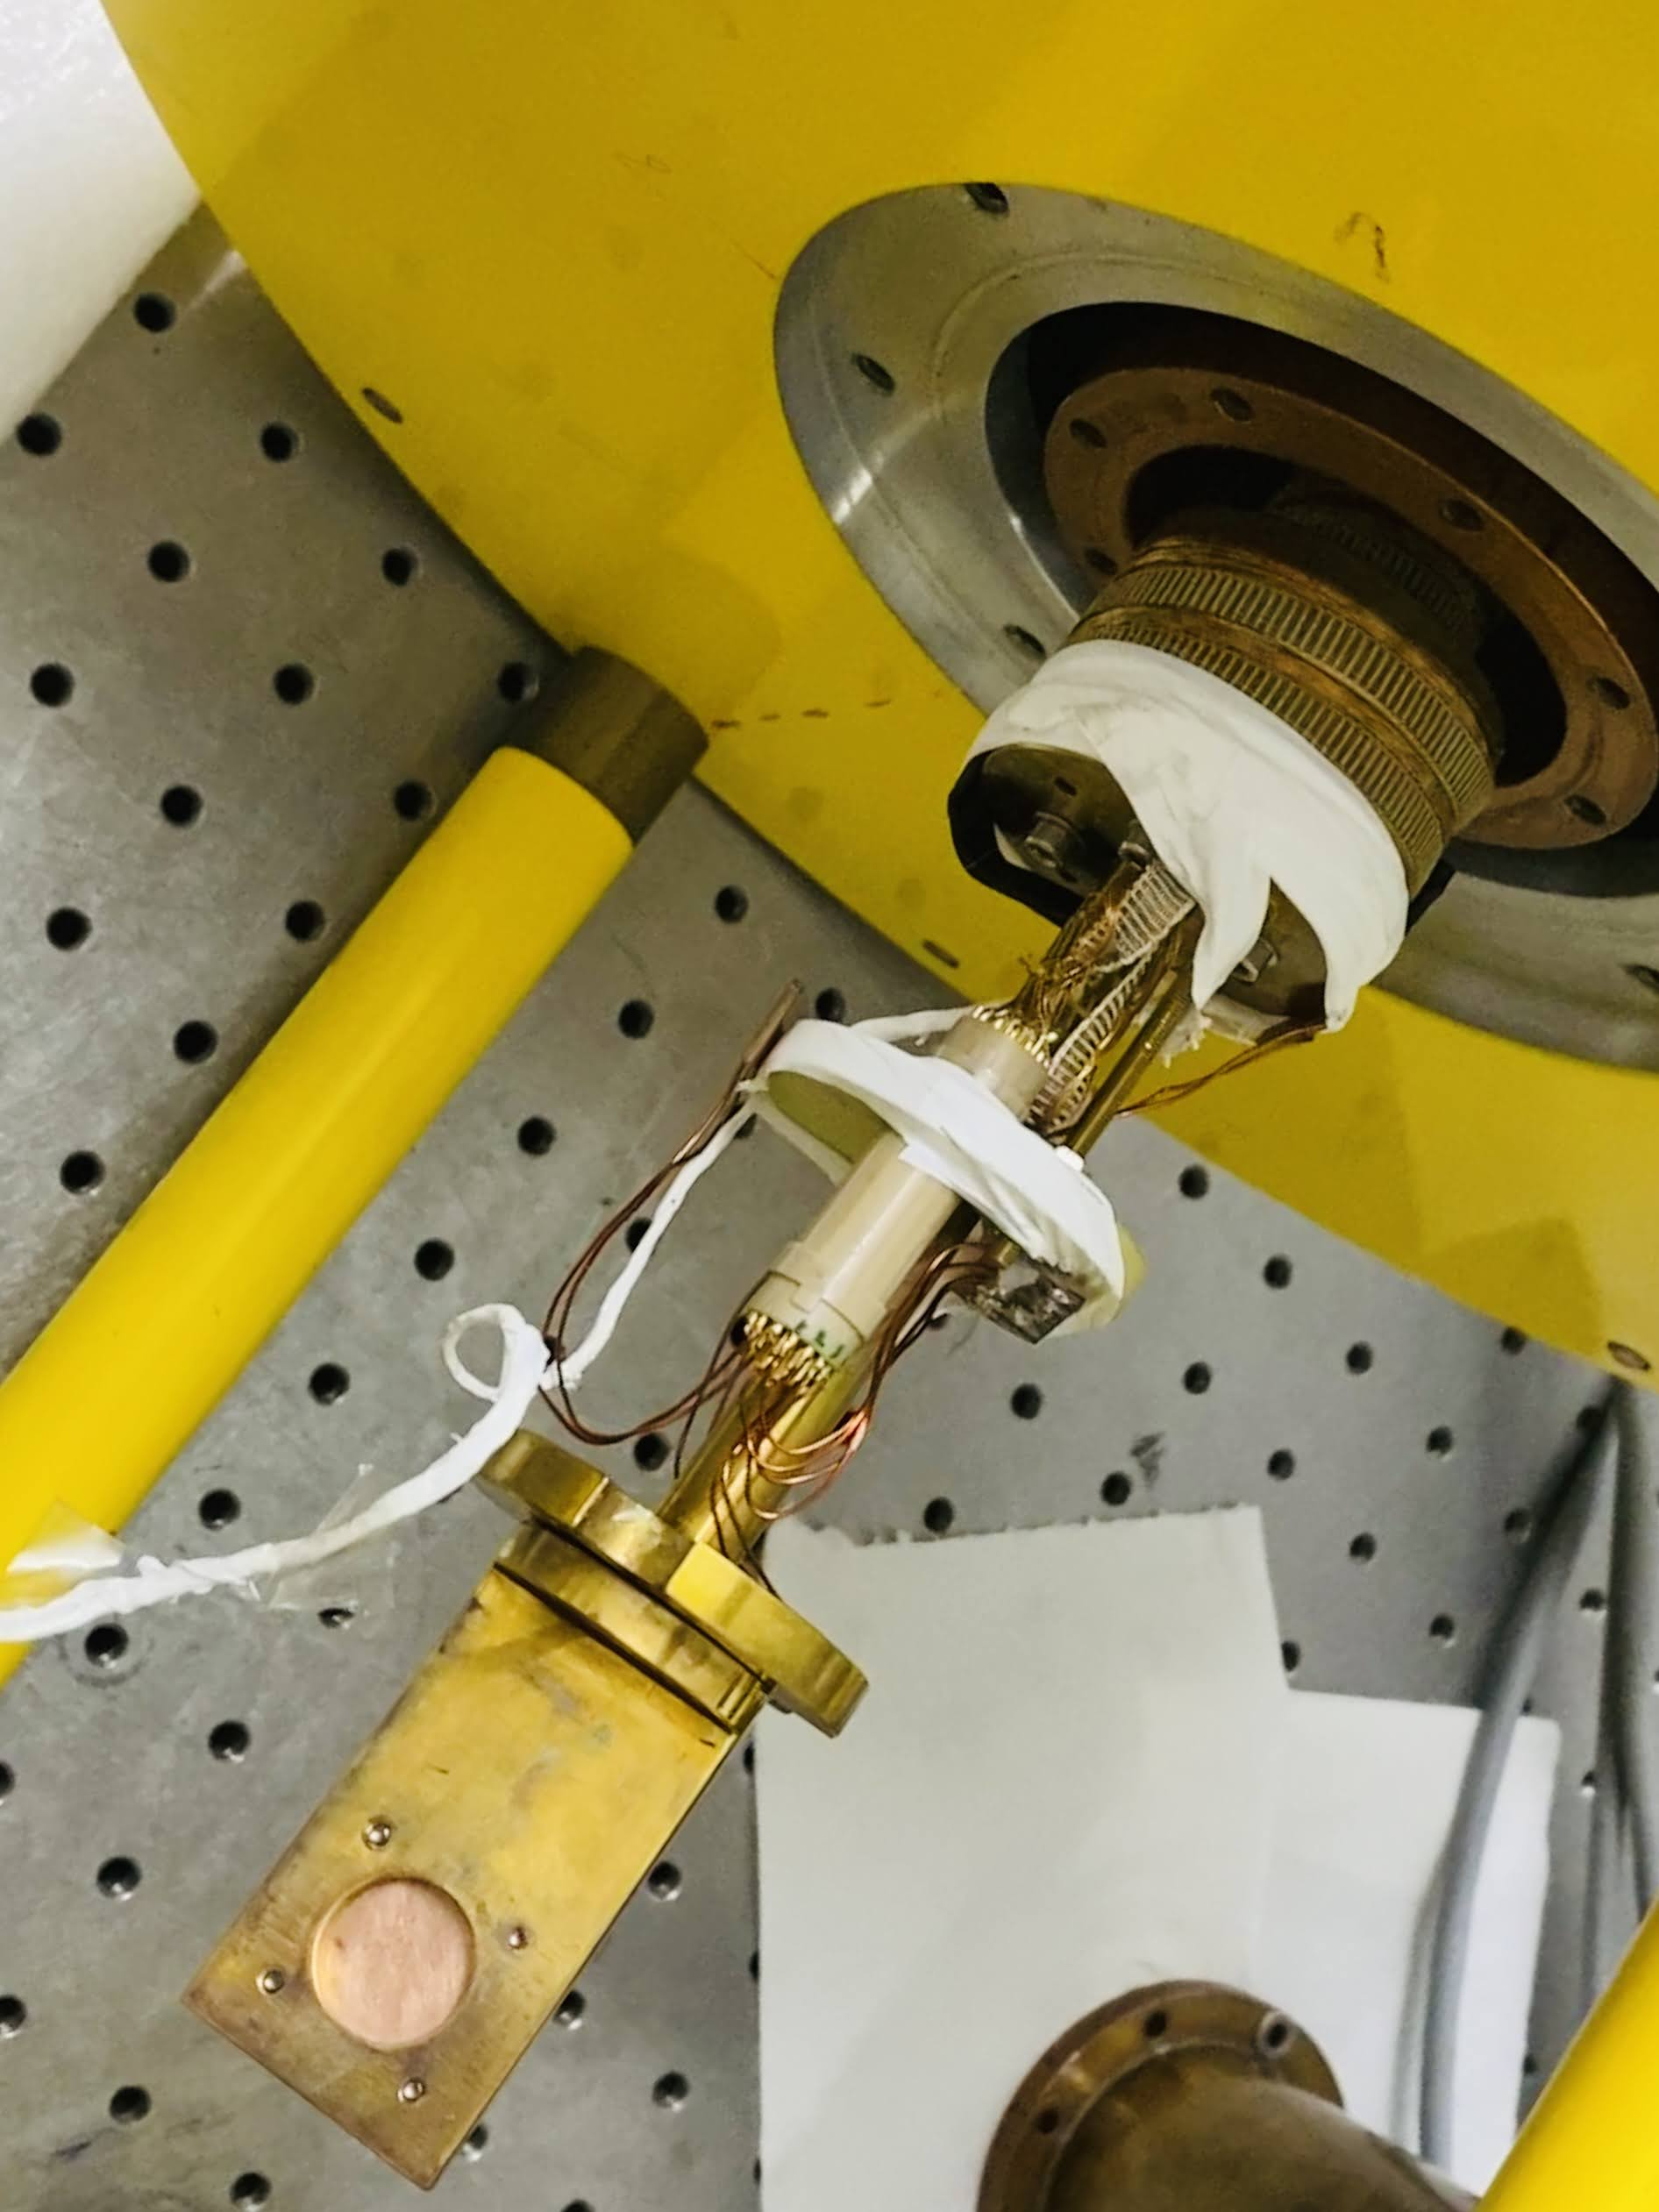}
    \caption{Inside of cryostat}
    \label{fig:first}
\end{subfigure}
\hfill
\begin{subfigure}{0.5\textwidth}
    \includegraphics[width=\textwidth]{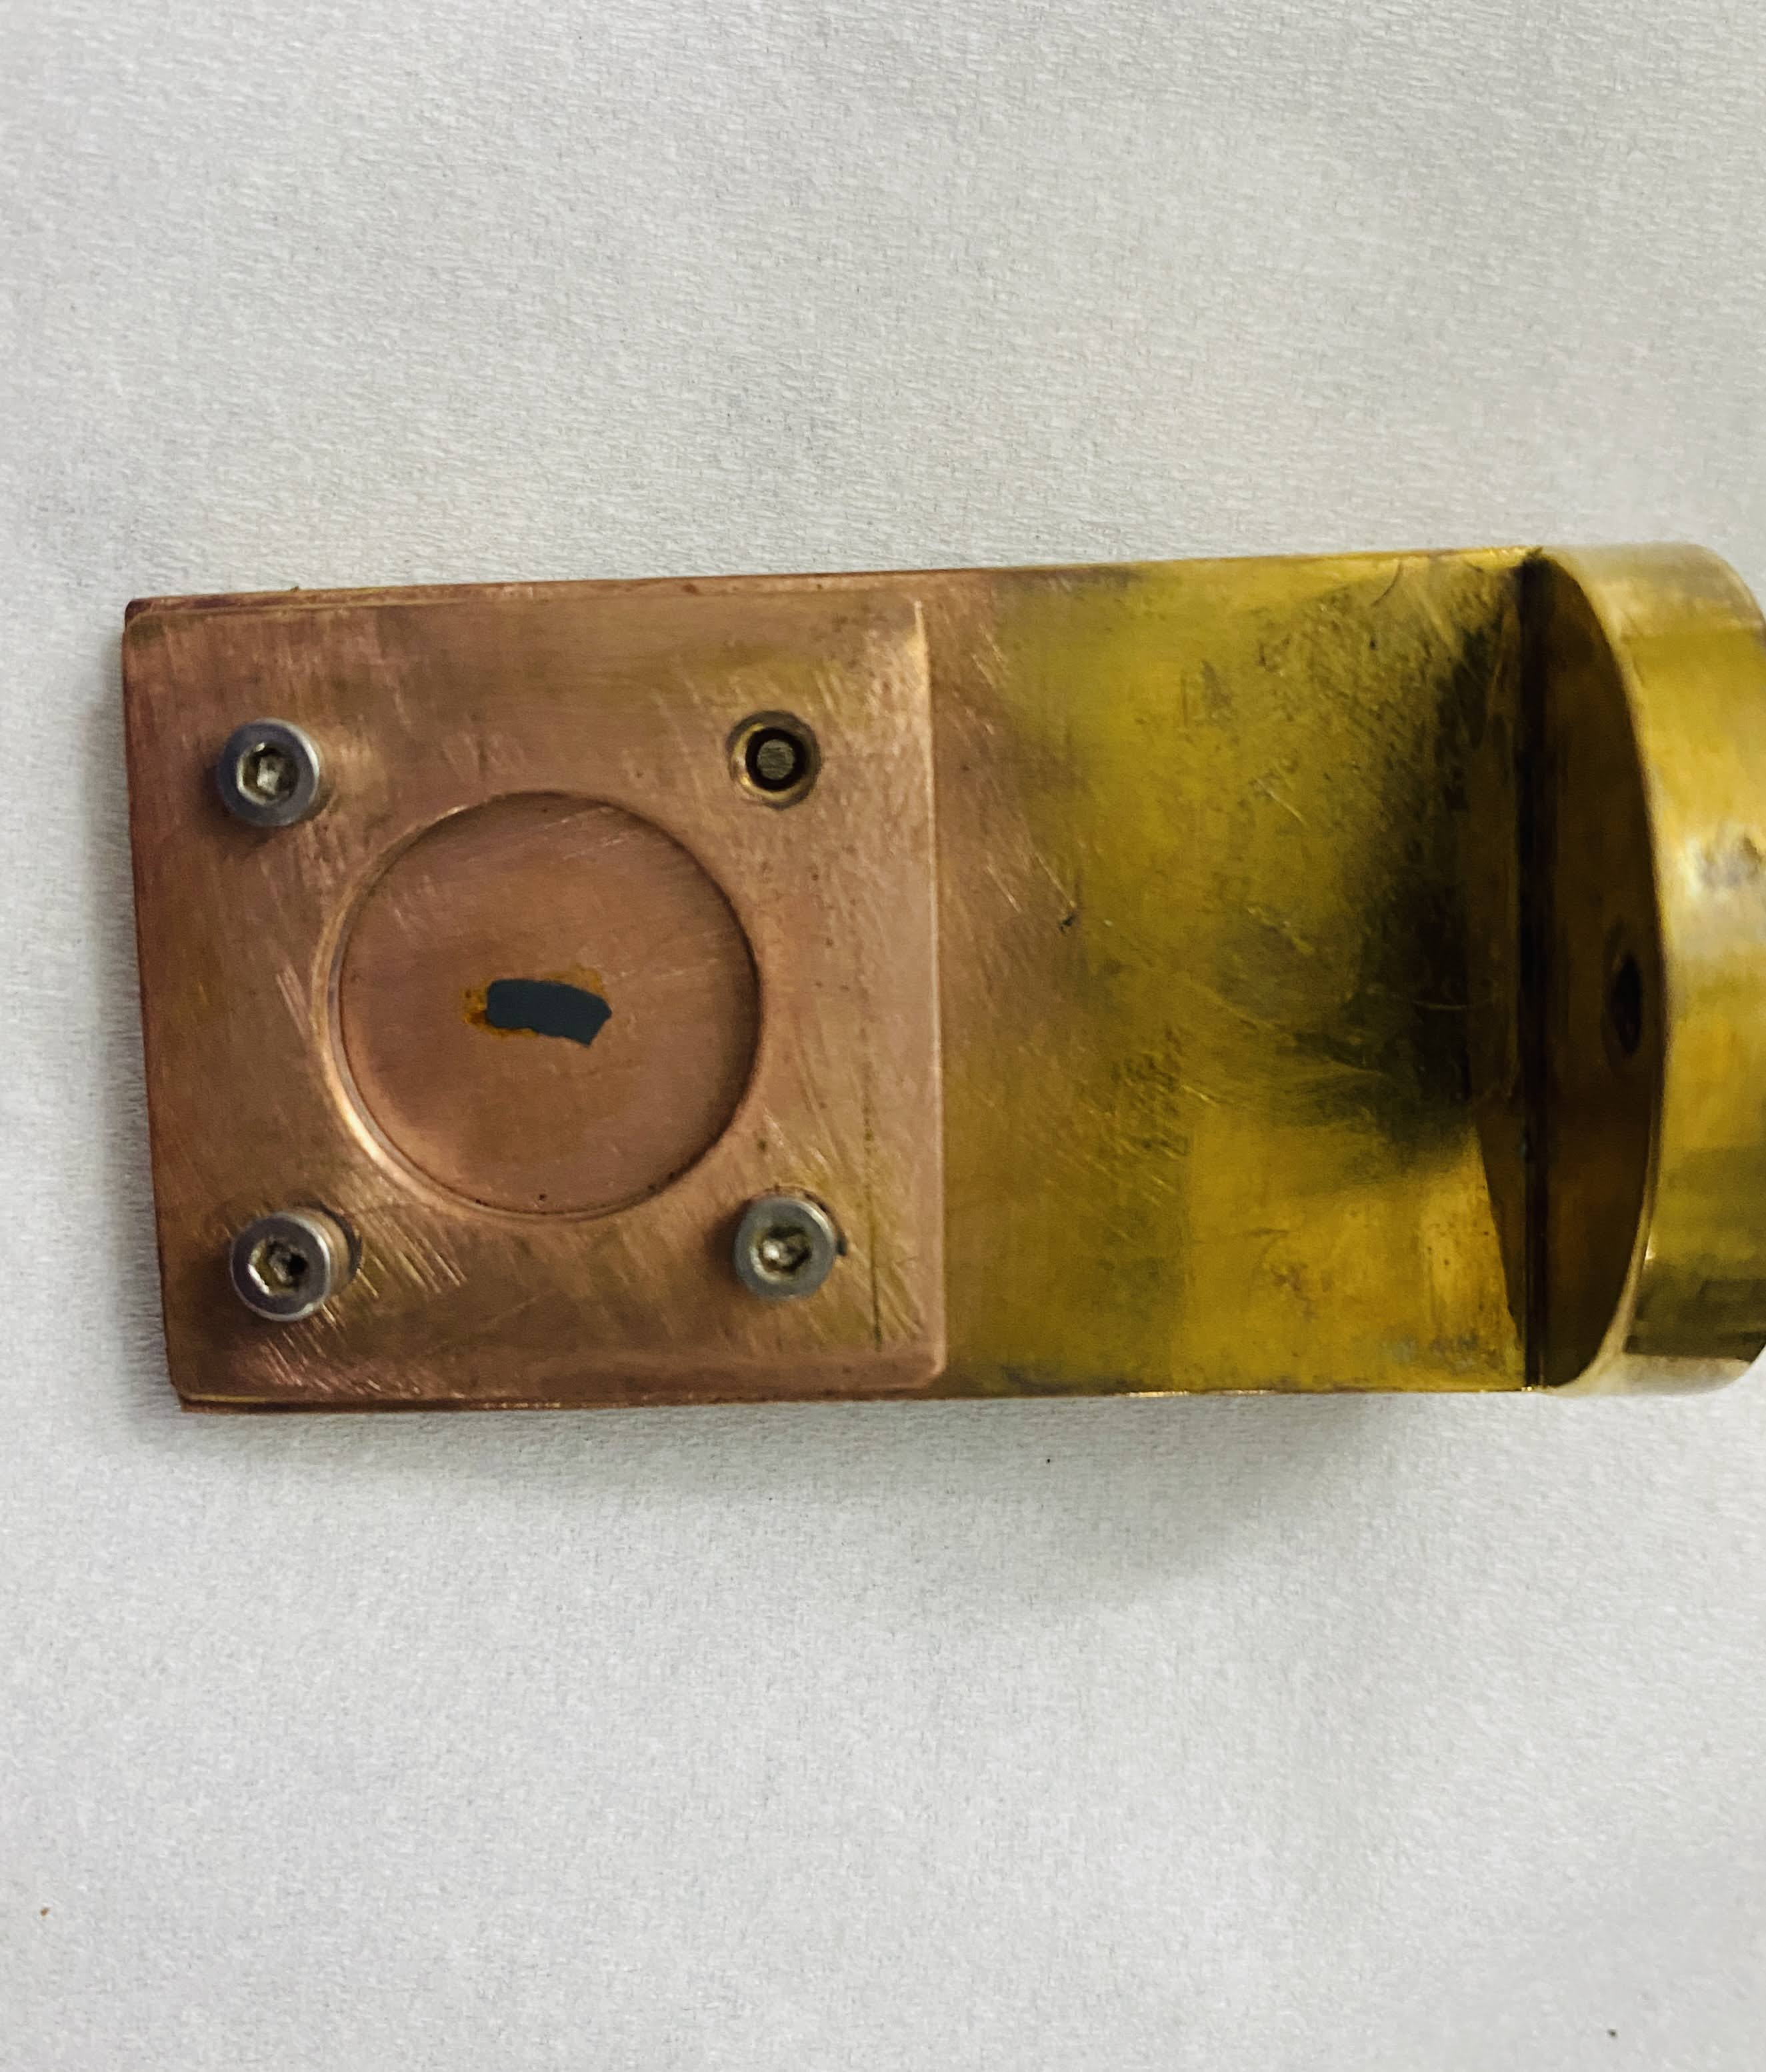}
    \caption{Sample holder}
    \label{fig:second}
\end{subfigure}
\hfill
        
\caption{Interior of cryostat}
\label{fig:figures}
\end{figure}

\begin{figure}[h]
\begin{subfigure}{0.38\textwidth}
    \includegraphics[width=\textwidth]{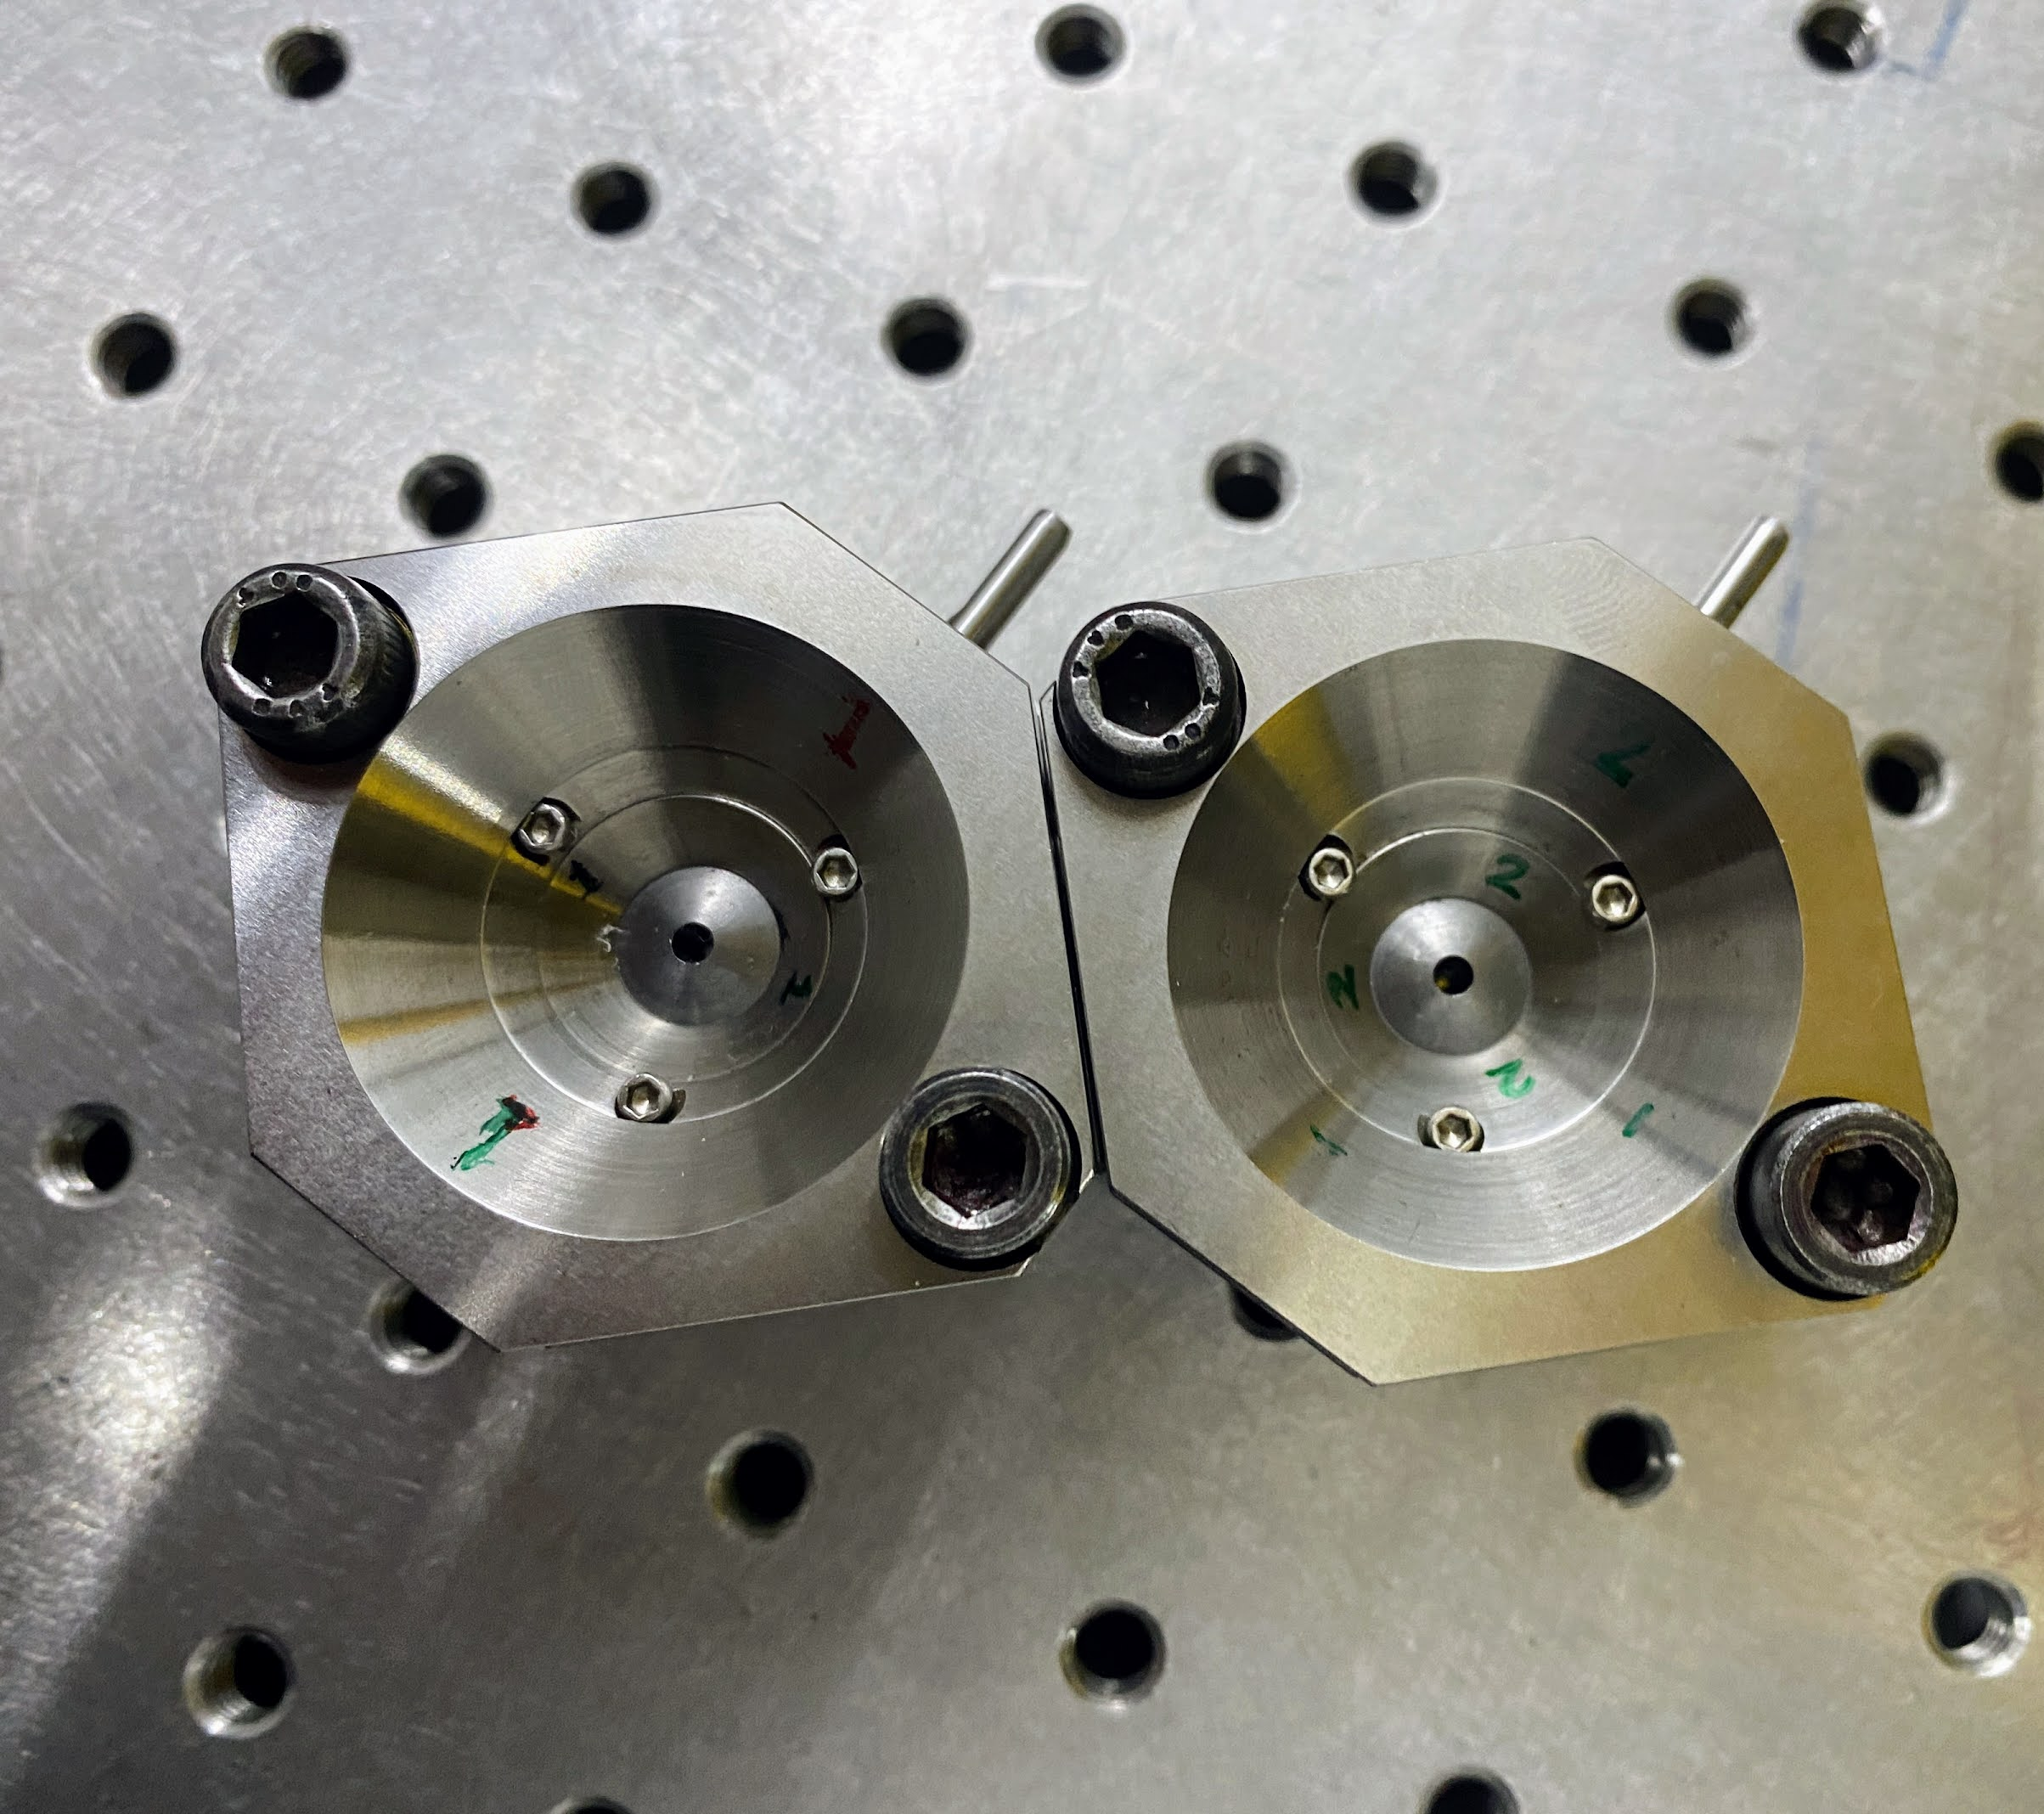}
    \caption{Top view of DAC}
    \label{fig:first}
\end{subfigure}
\hfill
\begin{subfigure}{0.5\textwidth}
    \includegraphics[width=\textwidth]{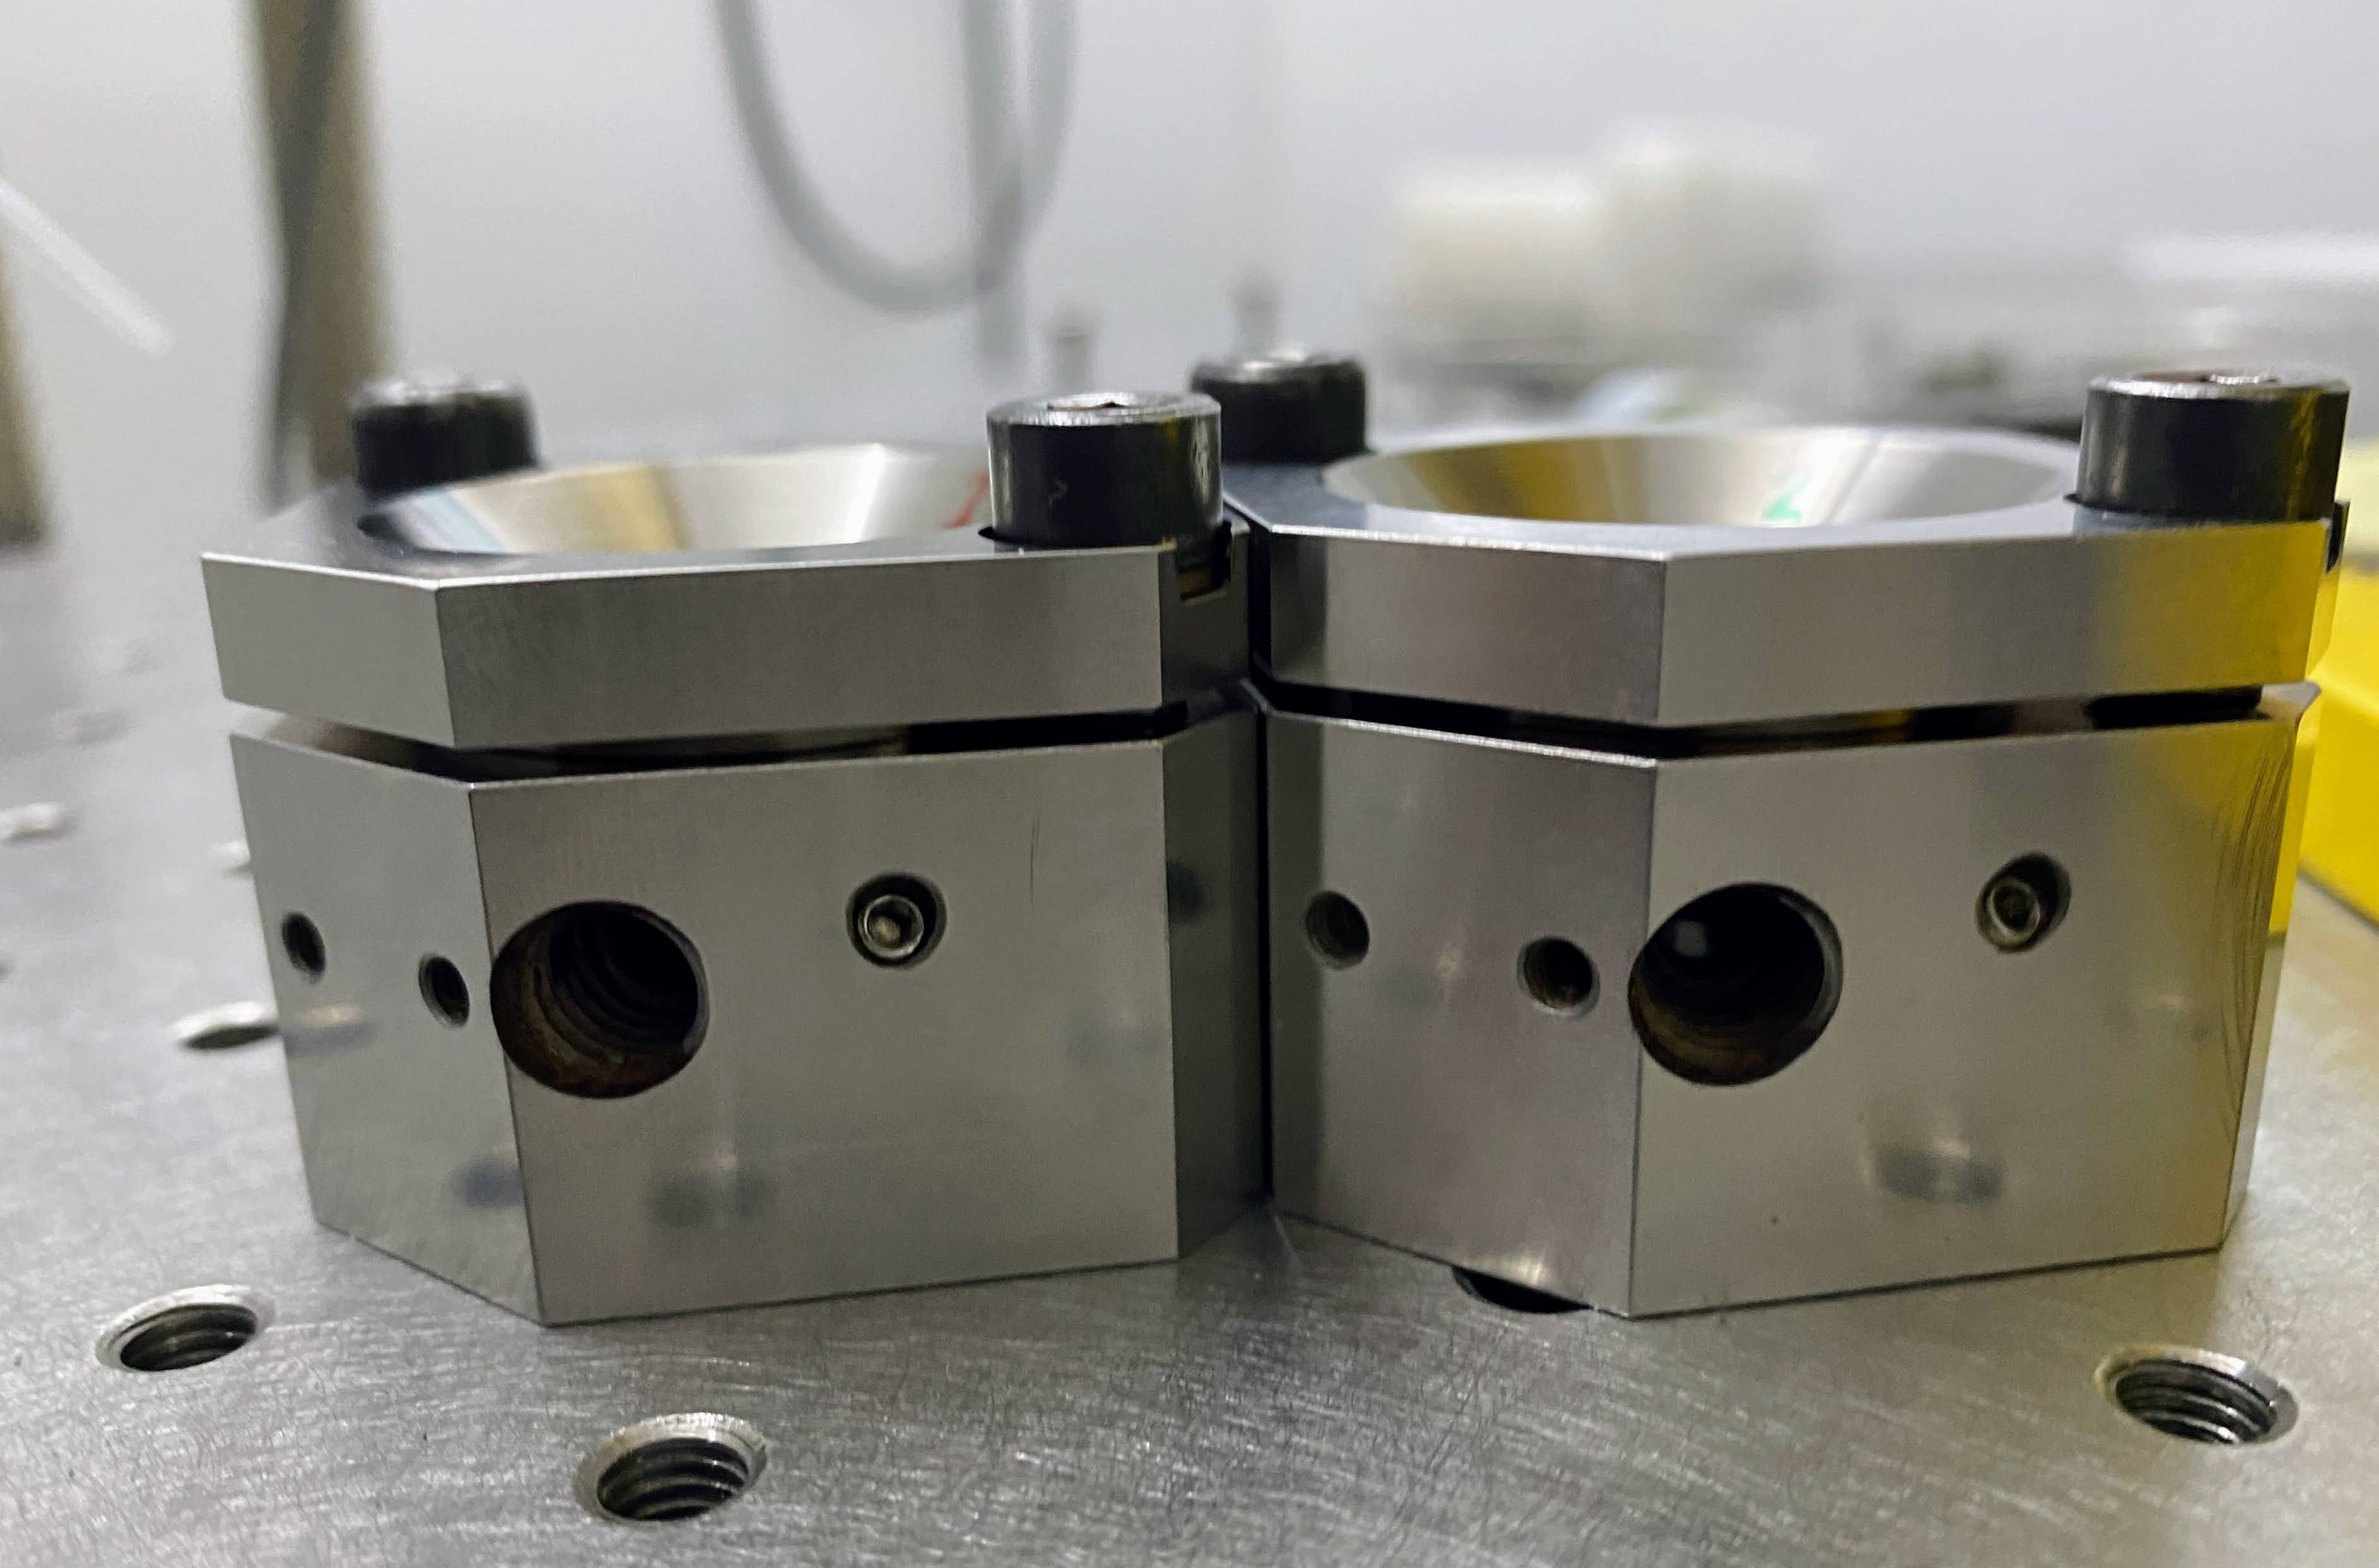}
    \caption{Side view DAC}
    \label{fig:second}
\end{subfigure}
\hfill
        
\caption{Top and Side view of Diamond Anvil Cell}
\label{fig:figures}
\end{figure}

\chapter{Tables and Graphs}

\begin{figure}[h]
\centering
\begin{subfigure}{0.49\textwidth}
    \includegraphics[width=\textwidth]{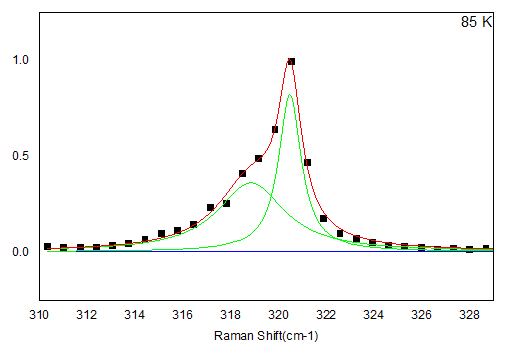}
    \caption{Peak splitting in Cs$_2$TiCl$_6$ (3\% Sb) system}
    \label{fig:first}
\end{subfigure}
\hfill
\begin{subfigure}{0.49\textwidth}
    \includegraphics[width=\textwidth]{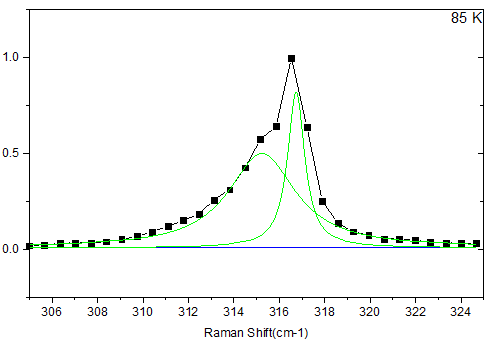}
    \caption{Peak splitting in Cs$_2$Ti$_{(1-x)}$Sb$_x$Cl$_6$ (x=2\%) system}
    \label{fig:second}
\end{subfigure}
\hfill
        
\caption{Peak splitting in at Cs$_2$TiCl$_6$ (3\% Sb) and Cs$_2$Ti$_{(1-x)}$Sb$_x$Cl$_6$ (x=2\%) at less than 100K}
\label{fig:figures}
\end{figure}

\begin{table}[H]
    \centering   
\begin{tabular}{ |p{3cm}||p{3cm}|p{3cm}|p{3cm}|  }
 \hline
Raman Modes & Peak Position at 267 K (cm$^{-1}$) & Peak Position at 22 K (cm$^{-1}$) & Change in peak position $\Delta x_c$  \\
 \hline
 Bending T$_{2g}$  & 184.4   & 185.31 & 0.91  \\
 
Stretching A$_{1g}$& 319.54   & 322.29 & 2.75 \\
 \hline
\end{tabular}
\caption{Shift in the peak position of identified Raman modes with temperature in Cs$_2$TiCl$_6$ system}
    \label{tab:my_label}
\end{table}

\begin{table}[H]
    \centering   
\begin{tabular}{ |p{3cm}||p{3cm}|p{3cm}|p{2.5cm}|}
 \hline
Raman Modes & FWHM at 267 K (cm$^{-1}$) & FWHM at 22 K (cm$^{-1}$) & Change in FWHM    \\
 \hline
 Bending T$_{2g}$  & 6.16  & 3.96 & 2.2   \\
 
Stretching A$_{1g}$& 6.36   & 3.99 & 2.37 \\
 \hline
\end{tabular}
\caption{Change in FWHM of identified Raman modes with temperature in Cs$_2$TiCl$_6$ system }
    \label{tab:my_label}
\end{table}

\begin{table}[H]
    \centering   
\begin{tabular}{ |p{3cm}||p{3cm}|p{3cm}|p{3cm}|  }
 \hline
Raman Modes & Peak Position at 300 K (cm$^{-1}$) & Peak Position at 22 K (cm$^{-1}$) & Change in peak position $\Delta x_c$  \\
 \hline

Translational T${2_g}$ & 51.62   & 54.37 & 2.75 \\
 
Bending T$_{2g}$  & 181.98   & 183.35 & 1.37  \\
 
Stretching A$_{1g}$& 316.53   & 320.6 & 4.07 \\
 \hline
\end{tabular}
\caption{Shift in the peak position of identified Raman modes with temperature in Cs$_2$TiCl$_6$  (3\% Sb) system }
    \label{tab:my_label}
\end{table}

\begin{table}[H]
    \centering   
\begin{tabular}{ |p{3cm}||p{3cm}|p{3cm}|p{3cm}|  }
 \hline
Raman Modes & FWHM at 267 K (cm$^{-1}$) & FWHM at 22 K (cm$^{-1}$) & Change in FWHM    \\
 \hline
 Translational T${2_g}$ & 0.8   & 0.02 & 0.78 \\
 
Bending T$_{2g}$  & 5.1   & 2.34 & 2.76  \\
 
Stretching A$_{1g}$& 6.07   & 1.08 & 4.99 \\
 \hline
\end{tabular}
\caption{Change in FWHM of identified Raman modes with temperature in Cs$_2$TiCl$_6$ (3\% Sb) system }
    \label{tab:my_label}
\end{table}

\begin{table}[H]
    \centering   
\begin{tabular}{ |p{3cm}||p{3cm}|p{3cm}|p{3cm}|  }
 \hline
Raman Modes & Peak Position at 267 K (cm$^{-1}$) & Peak Position at 22 K (cm$^{-1}$) & Change in peak position $\Delta x_c$  \\
 \hline

Translational T${2_g}$ & 47.81   & 50.55 & 2.74 \\
 
Bending T$_{2g}$  & 178.18   & 179.65 & 1.47  \\

Stretching A$_{1g}$& 312.95   & 316.90 & 3.95  \\
 \hline
\end{tabular}
\caption{Shift in the peak position of identified Raman modes with temperature in Cs$_2$Ti$_{(1-x)}$Sb$_x$Cl$_6$ (x = 2\% ) system}
    \label{tab:my_label}
\end{table}

\begin{table}[H]
    \centering   
\begin{tabular}{ |p{3cm}||p{3cm}|p{3cm}|p{3cm}|  }
 \hline
Raman Modes & FWHM at 267 K (cm$^{-1}$) & FWHM at 22 K (cm$^{-1}$) & Change in FWHM    \\
 \hline
 Translational T${2_g}$ & 2.29   & 0.8484 &  \\
 
Bending T$_{2g}$  & 5.05   & 2.098 & 2.952  \\
 
Stretching A$_{1g}$& 5.88   & 0.4437 & 5.4363 \\
 \hline
\end{tabular}
\caption{Change in FWHM of identified Raman modes with temperature in Cs$_2$Ti$_{(1-x)}$Sb$_x$Cl$_6$ (x = 2\% ) system}
    \label{tab:my_label}
\end{table}

\begin{figure}[h]
\centering
\begin{subfigure}{0.3\textwidth}
    \includegraphics[width=\textwidth]{appendix/dacppt.png}
    \caption{Schematic of sample loaded DAC with ruby}
    \label{fig:first}
\end{subfigure}
\hfill
\begin{subfigure}{0.49\textwidth}
    \includegraphics[width=\textwidth]{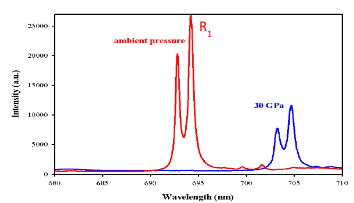}
    \caption{Peak splitting in Cs$_2$Ti$_{(1-x)}$Sb$_x$Cl$_6$ (x=2\%) system}
    \label{fig:second}
\end{subfigure}
\hfill
        
\caption{Fluorescence of Ruby at ambinet and 30GPa pressure}
\label{fig:figures}
\end{figure}
\begin{table}[H]
    \centering   
\begin{tabular}{ |p{3cm}||p{3cm}|p{3cm}|p{3cm}|  }
 \hline
Raman Modes & Peak position at 30 Gpa (cm$^{-1}$) & Peak position at Ambient Pressure (cm$^{-1}$) & Change in Peak position (cm$^{-1}$)    \\
 \hline
 
Bending T$_{2g}$  & 327.80    & 183.14  & 144.66  \\
 
Stretching A$_{1g}$& 475.28  & 317.74 & 157.54 \\
 \hline
\end{tabular}
\caption{Change in peak position of identified Raman modes with pressure in Cs$_2$Ti$_{(1-x)}$Sb$_x$Cl$_6$ (x = 2\% ) system}
    \label{tab:my_label}
\end{table}

\begin{table}[H]
    \centering   
\begin{tabular}{ |p{3cm}||p{3cm}|p{3cm}|p{3cm}|  }
 \hline
Raman Modes & slope & intercept & ($\chi ^2$)    \\
 \hline
 
Bending T$_{2g}$  & 4.90    & 195.16  & 0.9996  \\
 
Stretching A$_{1g}$& 4.93  & 322.64 & 0.9984 \\
 \hline
\end{tabular}
\caption{Slope and intercept of fitted peak position versus pressure graph of Cs$_2$Ti$_{(1-x)}$Sb$_x$Cl$_6$ (x = 2\% ) system}
    \label{tab:my_label}
\end{table}

\begin{table}[H]
    \centering   
\begin{tabular}{ |p{3cm}||p{3cm}|p{3cm}|p{3cm}|  }
 \hline
Pressure (GPa) & Peak position (cm$^{-1}$) & FWHM (cm$^{-1}$) & Area (a.u)    \\
 \hline
 
3.3  & 600.63    & 192.07 &339.31  \\
 
13.36 A$_{1g}$& 204.91  & 322.64 & 388.57 \\

31.92 A$_{1g}$& 277.05  & 322.64 & 376.17 \\
 
 \hline
\end{tabular}
\caption{Peak position evolution of PL spectra with increase in pressure of  Cs$_2$Ti$_{(1-x)}$Sb$_x$Cl$_6$ (x = 2\% ) system}
    \label{tab:my_label}
\end{table}
